# Supplementary material for: Quantum computation of molecular geometry via many-body nuclear spin echoes
Source: arXiv:2510.19550 source file (2025-10-22)

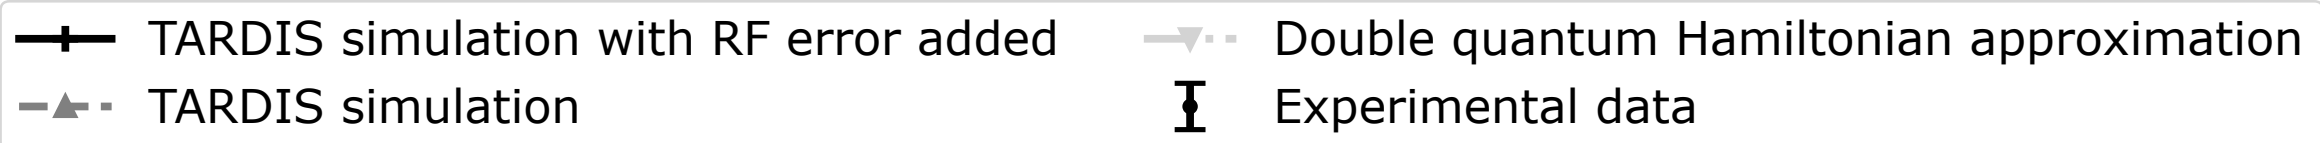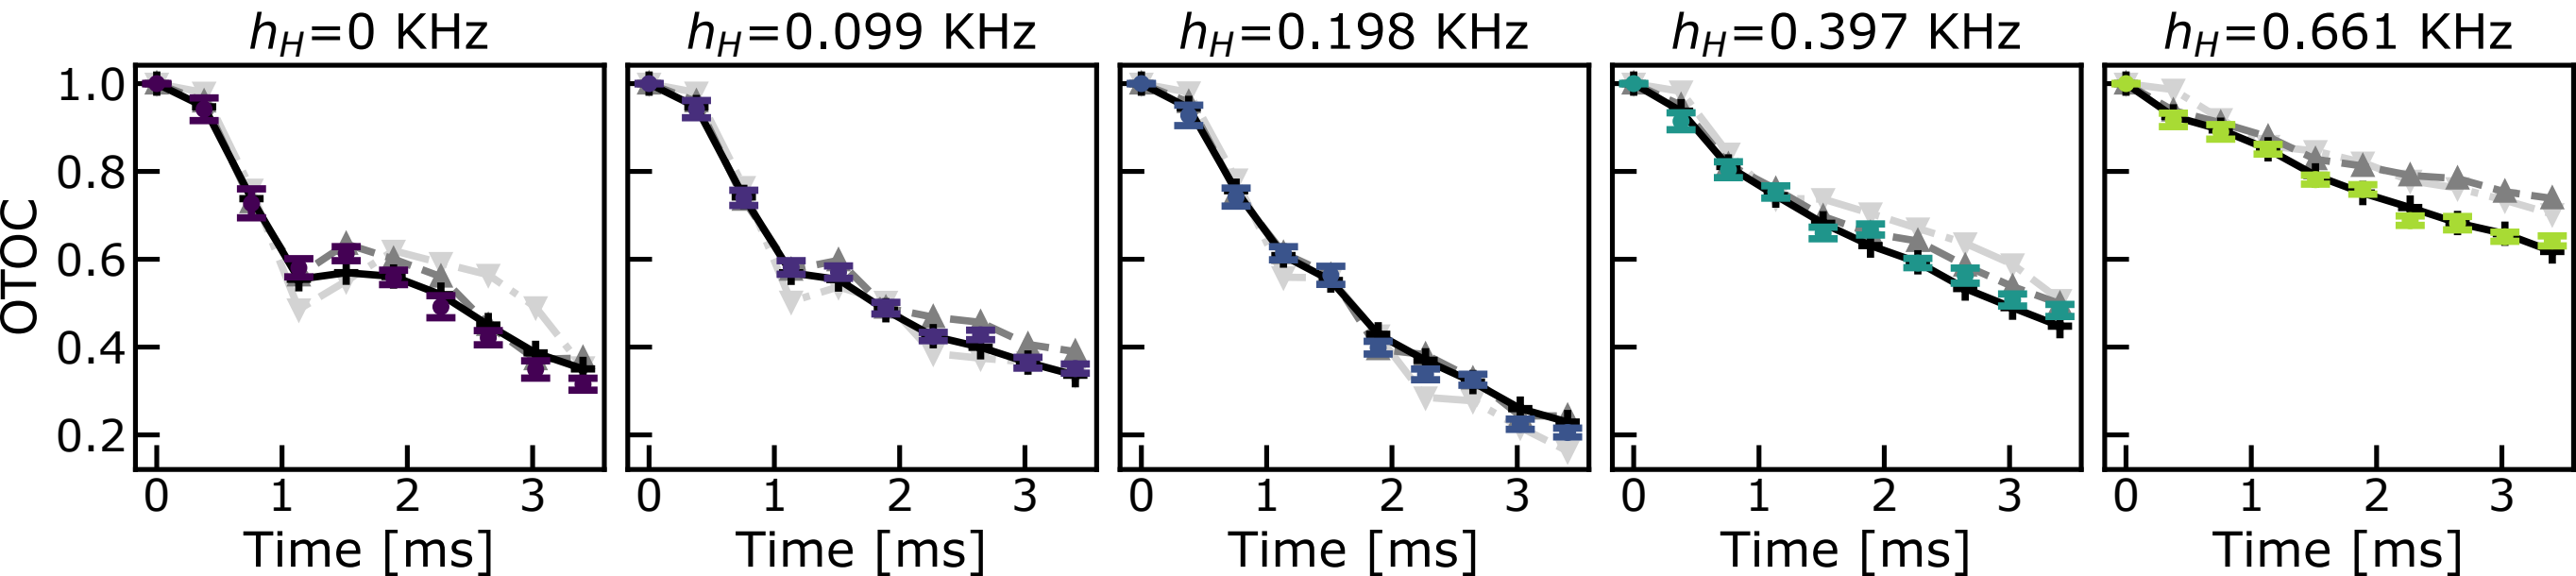

Supplement: Supplementary file 1 [file SM_all_toluene_otocs_with_fits.pdf]
